# Supplementary material for: Dual Dynamic Inference: Enabling More Efficient, Adaptive and Controllable Deep Inference
Source: arXiv:1907.04523 source file (2020-01-03)
Supplement: Supplementary file 1 [file 5-Supplementary.tex]

\onecolumn
\title{Supplementary Materials}
\vspace{0.9em}
\maketitle

In this supplementary material, Sec.\ref{one} provides the training details of the proposed DDI framework; Sec. \ref{two} shows the structure of the gating network of channel skipping in DenseNet； Sec. \ref{three} introduces the structure of branch classifiers of RADI; We show further visualization of feature maps under channel/ layer skipping, and the skipping ratio distributions of the two schemes at Sec. \ref{five}

\section{Training Details of DDI} \label{one}
\textbf{IADI Stage} The training of DDI framework has two stages. For the first IADI, we train it from a pre-trained base CNN model. If we directly start the training with randomly initialized gate networks using Gaussian distribution, the skipping ratio will be around 50\% from the beginning, which causes the mismatch between pre-trained batch normalization layers and unseen feature maps statistical distribution. To this end, we propose a warm-up process at the beginning to reduce the training instability caused by the mismatch. During the warm-up process, parameters in the base networks including batch normalization layers are fixed and only gate networks are trained to have zero skipping ratio. Then we use SGD as the optimizer to train the base network and gate networks end to end as described in the paper.

\textbf{DDI Stage} After the first stage is finished, we add intermediate branch classifiers to the well-trained IADI model, then train the whole DDI framework end to end as described in \ref{5}, the hyperparameters used for this stage is the same for IADI training.

\textbf{Hyperparameter Settings} For both CIFAR-10 and ImageNet datasets, We set momentum to 0.9, weight-decay to 1e-4. For CIFAR-10 experiments, we set learning rate to 5e-2, batch size to 128, $\alpha$ to 2e-4, for the IADI stage, we train a total of 50k iterations, for DDI stage, we train another 50k iterations. For ImageNet dataset, we set initial learning rate to 5e-2, batch size to 512, $\alpha$ to 4e-6, and similarly, we train IADI and DDI in sequential order, each with 90 epochs.

\section{Gating Design for DenseNet}\label{two}

As we discussed in Sec. \ref{2}, to reduce the prohibitive computational cost of gating network $G^C$ in DenseNet, we design a light weight gating network. Specifically, we construct the first two layers of the gating network in similar structure to a denselayer in DenseNet. By adjusting the stride and output channel number of the first 1x1 convolution layer, we can control the FLOPs of the gating network, and we experimentally found out that when the FLOPs of the gating network are around 11 \% of that of the denselayer, the channel skipping method in DenseNet achieves the best computation saving/accuracy tradeoff.

\begin{figure*}[ht]
\centering     %%% not \center
\subfigure[Structure of a Denselayer]{\label{fig:denselayer}\includegraphics[width=80mm]{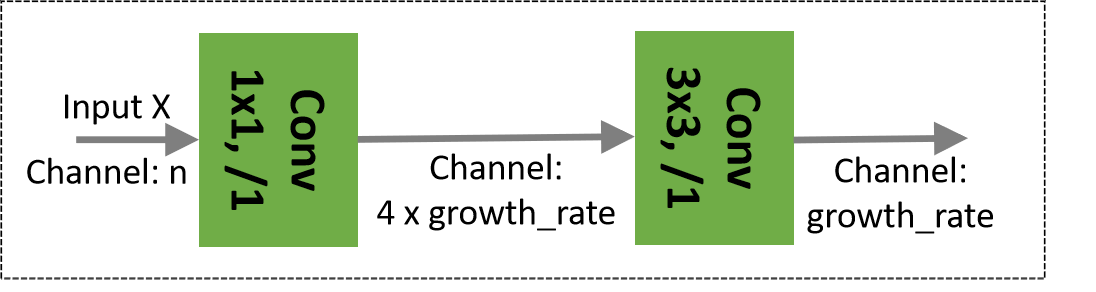}}
\subfigure[Structure of the proposed gating network]{\label{fig:gc_densenet}\includegraphics[width=80mm]{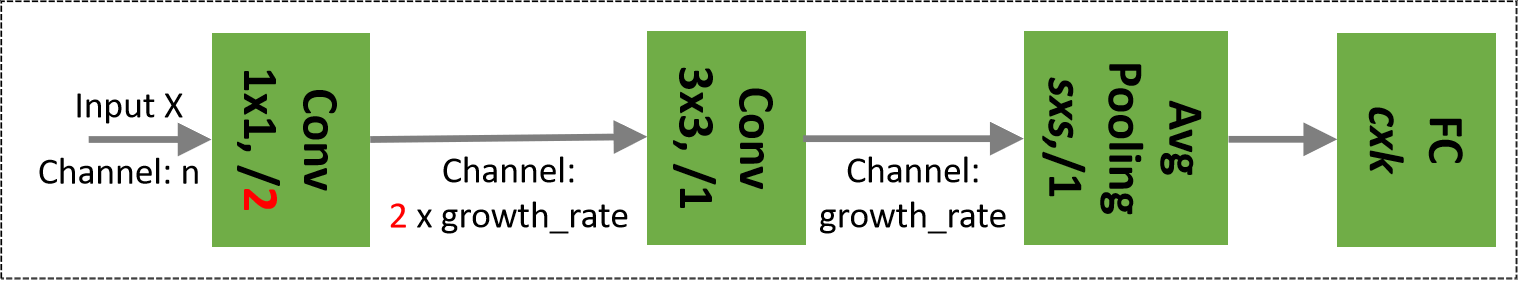}}
\vspace{-1.0em}
\caption{(a) Canonical denselayer structure in DenseNet. (b) The corresponding channel skipping gating network for (a). The first two layers of the gating network have similar structure of the denselayer in (a), the differences are that we change the stride of the first 1x1 convolution layer to 2 and decrease its output channel numbers by half. Note that by applying these modifications, the total FLOPs of the gating network is roughly 11 \% of that of a denselayer.}
\label{fig:gating_network}
% \vspace{-1em}
\end{figure*}

\section{RADI Branch Structure}\label{three}

Since in both ResNet and DenseNet architectures, the feature map size differs only between stages, we design the branch classifiers accordingly. Specifically, as shown in Fig. \ref{fig1:a}, in order to get coarse-grained features that is amenable for classification at early stage, the branch classifier has two max pooling layer at the first stage of the network. After that, the number of max pooling layer is decreased by one at second stage (Fig. \ref{fig1:b}), and for the third stage, the branch classifier consists of average pooling layer and fully connected layer only (Fig. \ref{fig1:c}).

\begin{figure}[!htb]
\minipage[b]{0.40\textwidth}
  \begin{subfigure}[\label{fig1:a}]
		\centering
		\includegraphics[width=17mm]{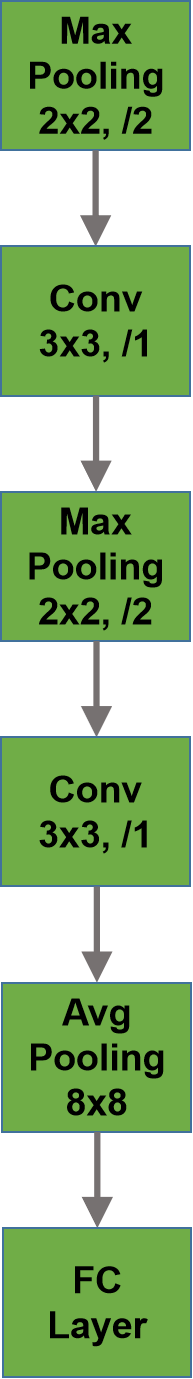}
	\end{subfigure}\hfill
    \begin{subfigure}[\label{fig1:b}]
		\centering
		\includegraphics[width=17mm]{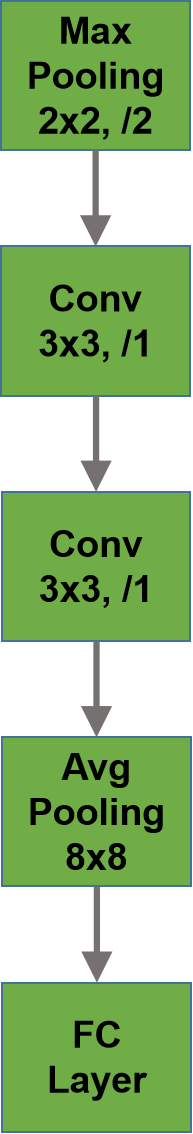}
	\end{subfigure}\hfill
	\begin{subfigure}[\label{fig1:c}]
		\centering
		\includegraphics[width=17mm]{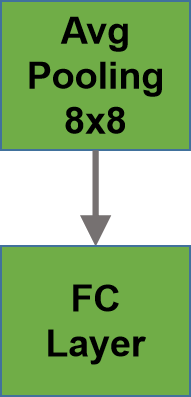}
	\end{subfigure}
	\caption{Branch classifier of: (a) stage one of the network, (b) stage two of the network, (c) stage three of the network}
  
\endminipage\hfill 
\minipage[b]{0.55\textwidth} 
  \includegraphics[width=100mm]{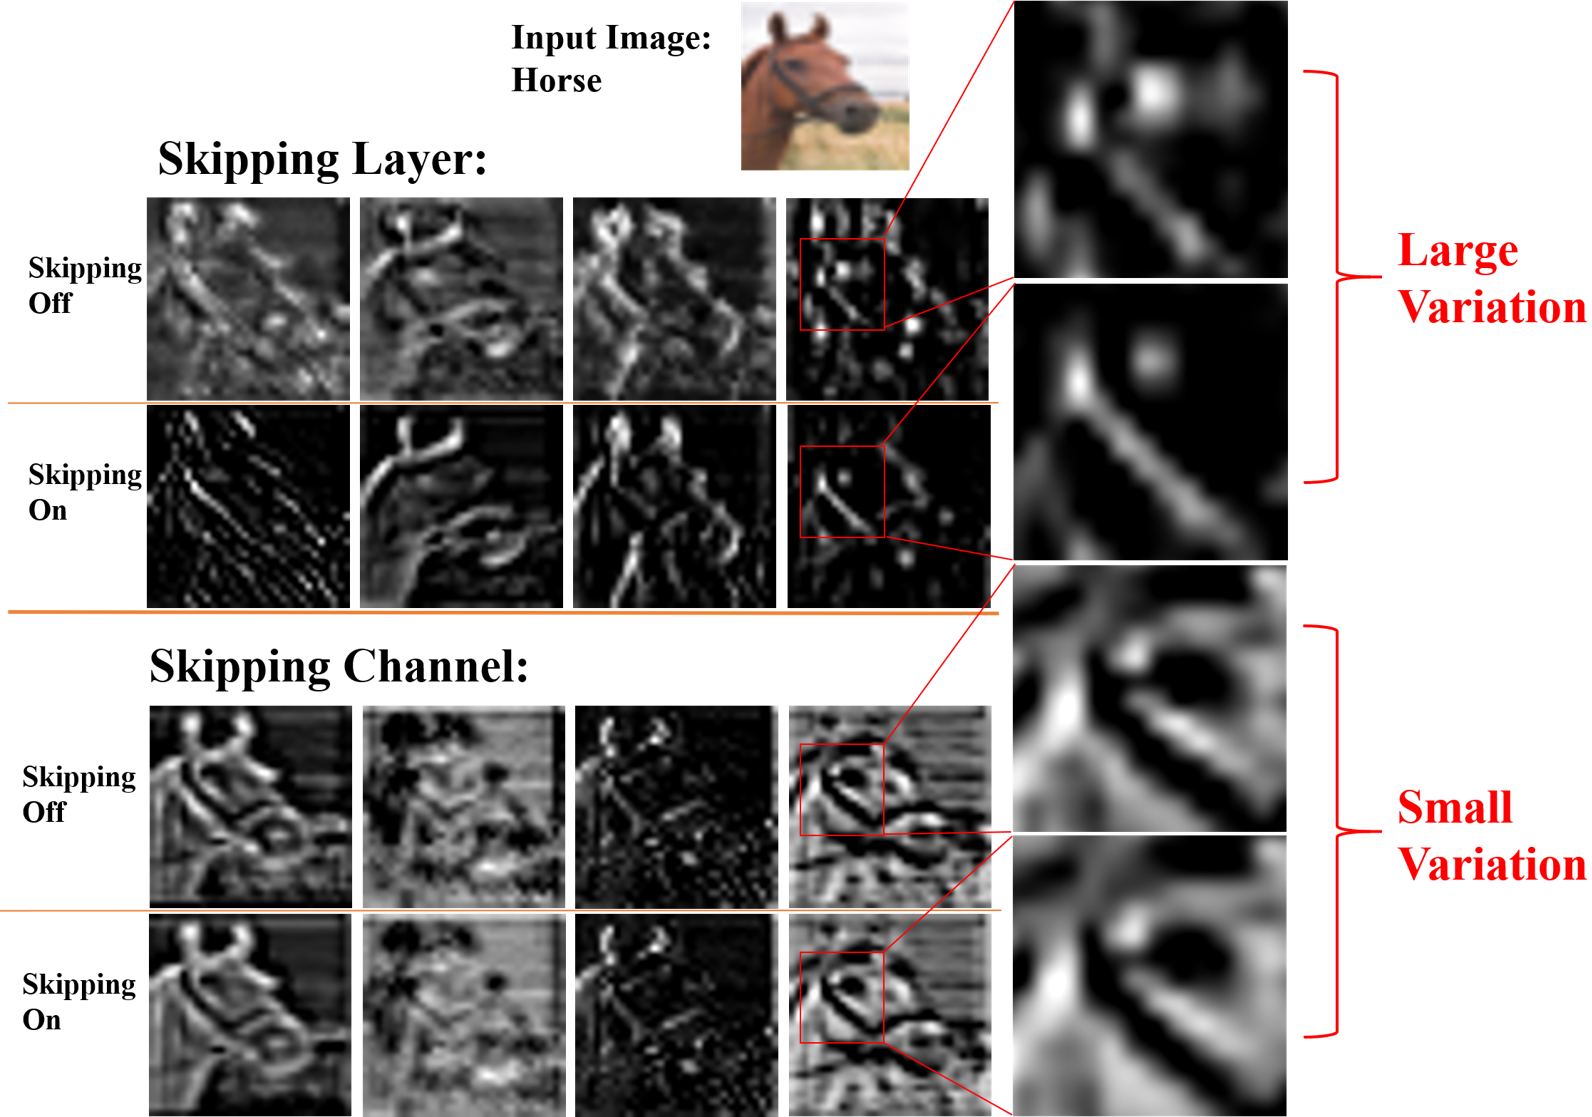}
  \caption{Visualizing feature degradation of layer/channel skipping (i.e., ``skipping on") over the original model (i.e., ``skipping off"), where the features are obtained from the 6th residual block when using ResNet38.}
\label{fig:fm_combo}
\endminipage\hfill

\end{figure}

\section{Detailed Skipping Behavior Visualization and Analysis} \label{five}

\textbf{Feature Degradation of Layer/Channel Skipping.}
We here visualize the feature degradation of layer/channel skipping compared with that of the original model. As shown in the example of Fig. \ref{fig:fm_combo}, layer skipping can cause feature change and large variation in terms of illumination sharpness and clarity, as compared with that of the original one, whereas the feature change and variation is marginal for channel skipping. This justifies the more gradual accuracy loss (see Fig. \ref{fig:savings}) offered by channel skipping than layer skipping under the same computational cost. 
% Then we compare intermediate feature maps of the learned model with skipping and the same model with 100\% executing rate, to analyze the influence of the skipping layer and skipping channel respectively. From Fig. \ref{fig:fm_combo}, we observe the feature maps of skipping layer model have large variation between Skipping On and Off in terms of sharpness and clarity. But for the model with finer-grained skipping channel, the nuance between opening and closing skipping is almost negligible. This less disturbance to feature maps of the skipping channel method explains the reason why it has higher accuracy than skipping layer method.

\begin{figure}[ht]
\vspace{-0.5em}
\begin{center}
\centerline{\includegraphics[width=\columnwidth]{Images/fm_combo.png}}
\vspace{-0.5em}
\caption{{Visualizing feature degradation of layer/channel skipping (i.e., ``skipping on") over the original model (i.e., ``skipping off"), where the features are obtained from the 6th residual block when using ResNet38.}
\label{fig:fm_combo}}
\end{center}
%  \vspace{-2.5em}
\end{figure}

\begin{figure*}[ht]
\vspace{-1em}
\begin{center}
\centerline{\includegraphics[width=500pt]{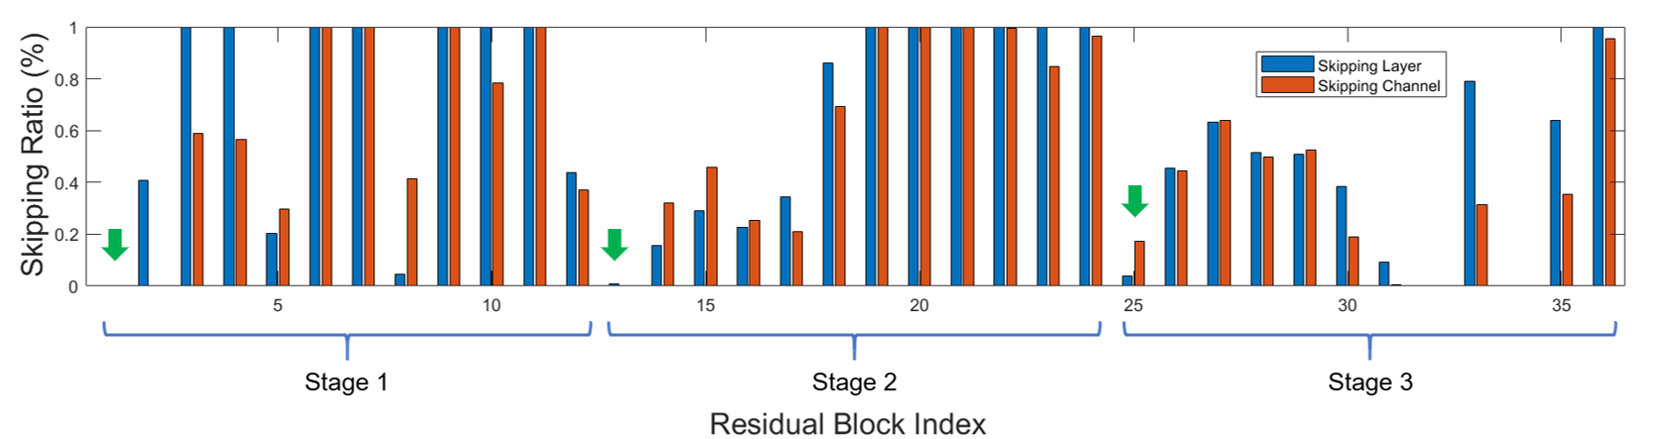}}
\caption{Visualizing the skipping patterns when applying layer/channel skipping to ResNet74 with both having an accuracy of about 92\% and 50\% computational saving, where there are 36 residual blocks divided into 3 stages uniformly. The first layer of each stage is marked with a green arrow.}
\label{fig:skipping_ratio}
\end{center}
\vspace{-2.5em}
\end{figure*}

\textbf{Skipping Patterns of Layer/Channel Skipping.} To visualize the effectiveness of layer/channel skipping, we show in Fig. \ref{fig:skipping_ratio} the skipping ratio of all the layers in ResNet74 when applying layer and channel skipping with both having a 92\% accuracy and 50\% computational savings. \cite{veit2016residual} has shown that while it is possible to skip most of the residual blocks except the first one at each stage for maintaining the accuracy. It is interesting to observe in Fig. \ref{fig:skipping_ratio} that both layer and channel skipping automatically learn the importance of the first residual block at each stage and avoid skipping them.
